# Supplementary material for: Detection of trade in products derived from threatened species using machine learning and a smartphone application
Source: arXiv:2509.06585 source file (2026-10-28)
Supplement: Supplementary file 1 [file Supplementary.tex]

\documentclass{article}
\usepackage[utf8]{inputenc}
\usepackage{authblk}
\usepackage{setspace}
\usepackage[margin=1.25in]{geometry}
\usepackage{graphicx}
\graphicspath{ {./figures/} }
\usepackage{subcaption}
\usepackage{amsmath}
\usepackage{lineno}
\usepackage{hyperref}
\usepackage{multirow}
%\linenumbers

\title{Supplementary: Detection of trade in products derived from threatened species using machine learning and a smartphone}
\author{}
\author[1*$\dag$]{Ritwik Kulkarni}
\author[3*]{WU Hanqin}
\author[1,2]{Enrico Di Minin}
\author[2]{Author Three}
\author[1,2]{Author Four}

%%%%%% Affiliations %%%%%%
\affil[1]{Helsinki Lab of Interdisciplinary Conservation Science, Department of Geosciences and
Geography, FI-00014, University of Helsinki, Finland}
\affil[2]{School of Life Sciences, University of KwaZulu-Natal, Durban 4041, South Africa}
\affil[3]{International Fund for Animal Welfare (IFAW)}
\date{}
\newcommand{\beginsupplement}{%
        \setcounter{table}{0}
        \renewcommand{\thetable}{ST\arabic{table}}%
        \setcounter{figure}{0}
        \renewcommand{\thefigure}{SF\arabic{figure}}%
     }

\begin{document}
\maketitle
\beginsupplement

\begin{table}[h]
    \centering
    \begin{tabular}{|c c c c c|}
    \hline
     & \multicolumn{1}{c}{\emph{Cross-entropy loss}} & &  & \\
    \hline
     & \multicolumn{2}{|c|}{mAP\_50} & \multicolumn{2}{|c|}{0.60}  \\
    \hline
     & \multicolumn{2}{|c|}{mAR\_100} & \multicolumn{2}{|c|}{0.56}  \\
    \hline
        Category & Elephant & Tiger & Pangolin & Non-Wildlife \\
        \hline
        Category wise mAP & 0.67   & 0.517  & 0.50  & 0.62 \\
        Category wise mAR & 0.75   & 0.68  & 0.62  & 0.72 \\
        Accuracy (\%) & 71.15    & 90.26  & 93.57  & 82.10\\
    \hline
     & \multicolumn{1}{c}{Asymmetric Focal loss} & & & \\
    \hline
     & \multicolumn{2}{|c|}{mAP\_50} & \multicolumn{2}{|c|}{0.40}  \\
    \hline
     & \multicolumn{2}{|c|}{mAR\_100} & \multicolumn{2}{|c|}{0.59}  \\
    \hline
        Category & Elephant & Tiger & Pangolin & Non-Wildlife \\
        \hline
        Category wise mAP & 0.61   &  0.33 & 0.06  & 0.56 \\
        Category wise mAR & 0.79 & 0.71 & 0.66 & 0.77 \\
        Accuracy (\%) & 30.67 & 9.18 & 3.25 & 51.70 \\
    \hline
    \end{tabular}
    \caption{Performance metrics on single model trained for all three species together}
    \label{tab:all_species}
\end{table}

\begin{table}[h!]
    \centering
    \begin{tabular}{|c c c |}
    \hline
     & \multicolumn{1}{c}{\emph{Cross-entropy loss}} &  \\
    \hline
     & \multicolumn{1}{|c|}{mAP\_50} & \multicolumn{1}{|c|}{0.53}  \\
    \hline
     & \multicolumn{1}{|c|}{mAR\_100} & \multicolumn{1}{|c|}{0.50}  \\
    \hline
        Category & Elephant Product  & Non-Wildlife \\
        \hline
        Category wise mAP & 0.68  & 0.60  \\
        Category wise mAR &  0.77  &  0.52 \\
        Accuracy (\%) &   65.04  &  78.25 \\
    \hline
     & \multicolumn{1}{c}{Asymmetric Focal loss} & \\
    \hline
     & \multicolumn{1}{|c|}{mAP\_50} & \multicolumn{1}{|c|}{0.51}  \\
    \hline
     & \multicolumn{1}{|c|}{mAR\_100} & \multicolumn{1}{|c|}{0.52}  \\
    \hline
        Category & Elephant Product & Non-Wildlife \\
        \hline
        Category wise mAP & 0.68   & 0.59   \\
        Category wise mAR & 0.79 &  0.76 \\
        Accuracy (\%) & 50.01 & 46.03  \\
    \hline
    \end{tabular}
    \caption{Performance metrics of single model trained on Elephant data}
    \label{tab:elephant}
\end{table}

\begin{table}[h!]
    \centering
    \begin{tabular}{|c c c |}
    \hline
     & \multicolumn{1}{c}{\emph{Cross-entropy loss}} &  \\
    \hline
     & \multicolumn{1}{|c|}{mAP\_50} & \multicolumn{1}{|c|}{0.50}  \\
    \hline
     & \multicolumn{1}{|c|}{mAR\_100} & \multicolumn{1}{|c|}{0.45}  \\
    \hline
        Category & Pangolin Product  & Non-Wildlife \\
        \hline
        Category wise mAP & 0.54   & 0.58  \\
        Category wise mAR & 0.66   & 0.70  \\
        Accuracy (\%) & 70.63    & 70.34  \\
    \hline
     & \multicolumn{1}{c}{Asymmetric Focal loss} & \\
    \hline
     & \multicolumn{1}{|c|}{mAP\_50} & \multicolumn{1}{|c|}{0.43}  \\
    \hline
     & \multicolumn{1}{|c|}{mAR\_100} & \multicolumn{1}{|c|}{0.45}  \\
    \hline
        Category & Pangolin Product & Non-Wildlife \\
        \hline
        Category wise mAP & 0.42   &  0.50  \\
        Category wise mAR & 0.66 & 0.71  \\
        Accuracy (\%) & 38.10 & 58.55  \\
    \hline
    \end{tabular}
    \caption{Performance metrics of single model trained on Pangolin data}
    \label{tab:pangolin}
\end{table}

\begin{table}[h!]
    \centering
    \begin{tabular}{|c c c |}
    \hline
     & \multicolumn{1}{c}{\emph{Cross-entropy loss}} &  \\
    \hline
     & \multicolumn{1}{|c|}{mAP\_50} & \multicolumn{1}{|c|}{0.51}  \\
    \hline
     & \multicolumn{1}{|c|}{mAR\_100} & \multicolumn{1}{|c|}{0.45}  \\
    \hline
        Category & Tiger Product  & Non-Wildlife \\
        \hline
        Category wise mAP & 0.53  & 0.61  \\
        Category wise mAR & 0.65   & 0.69  \\
        Accuracy (\%) & 82.70    & 78.78  \\
    \hline
     & \multicolumn{1}{c}{Asymmetric Focal loss} & \\
    \hline
     & \multicolumn{1}{|c|}{mAP\_50} & \multicolumn{1}{|c|}{0.49}  \\
    \hline
     & \multicolumn{1}{|c|}{mAR\_100} & \multicolumn{1}{|c|}{0.46}  \\
    \hline
        Category & Tiger Product & Non-Wildlife \\
        \hline
        Category wise mAP & 0.48   &  0.61  \\
        Category wise mAR & 0.66 & 0.71  \\
        Accuracy (\%) & 29.88 & 61.33  \\
    \hline
    \end{tabular}
    \caption{Performance metrics of single model trained on Tiger data}
    \label{tab:tiger}
\end{table}

\begin{figure}
    \centering
    \includegraphics[scale=0.2]{figures/tiger_inv.png}
    \caption{Represents  suspected tiger claws, and exhibits an anomalous activation pattern, with the Grad-CAM heatmap predominantly highlighting the surrounding background rather than the object itself.}
    \label{fig:inv_cam}
\end{figure}
\begin{figure}
    \centering
    \includegraphics[scale=0.5]{figures/examples.png}
    \caption{Examples of images from the database, spanning elephant, tiger and pangolin products identified by experts}
    \label{fig:enter-label}
\end{figure}

\begin{table}
    \centering
    \begin{tabular}{|cc|}
    \hline
        \textbf{Parameter} & \textbf{Value} \\
        \hline
        Number of Classes &  5 \\
        Learning Rate (initial) & 0.0001 (increased by 2x after performance plateau) \\
        Momentun & 0.9 \\
        Batch Size & 25 \\
        Epochs & 59 (CE and AFL) \\
        Stopping threshold & 15 \\
        Optimiser & ADAM \\
        Loss Function 1 & Cross-Entropy (CE) \\
        Loss Function 2 & Asymmetric Focal Loss (AFL)($\alpha = 0.25; \gamma = 2$)\\ 
        \hline
    \end{tabular}
    \caption{List of parameters used to train model}
    \label{tab:params_all}
\end{table}

\begin{table}
    \centering
    \begin{tabular}{|ccc|}
    \hline
        \textbf{Species Model} & \textbf{Epochs - CE}  & 
        \textbf{Epochs - AFL} \\
        \hline
        Elephant & 173 & 322\\
        Tiger & 54 & 265 \\
        Pangolin & 36 & 177\\
        \hline
    \end{tabular}
    \caption{Epochs of training for species specific models CE- Cross Entropy loss; AFL Asymmetric Focal loss}
    \label{tab:epochs_species}
\end{table}

\end{document}
